# Supplementary material for: Spin-glass-like behavior in the spin turbulence of spinor Bose-Einstein condensates
Source: arXiv:1304.4674 source file (2013-12-09)
Supplement: Supplementary file 1 [file supplement131120.pdf]

# Supplemental Material –Spin-glass-like behavior in the spin turbulence of spinor Bose-Einstein condensates–

Makoto Tsubota,[1,2] Yusuke Aoki,[1] and Kazuya Fujimoto[1]

[1] *Department of Physics, Osaka City University, Sumiyoshi-ku, Osaka 558-8585, Japan*
[2] *The OCU Advanced Research Institute for Natural Science and Technology (OCARINA), Osaka City University, Sumiyoshi-ku, Osaka 558-8585, Japan*

(Dated: December 9, 2013)

This document describes five topics for the spin turbulence not addressed in the manuscript: (I) interaction between components of energy, (II) dissipative mechanism in ST, (III) spectrum of kinetic energy, (IV) scale of energy injection and (V) magnitude of magnetization $|\boldsymbol{m}(t)|$.

PACS numbers: 03.75.Mn, 03.75.Kk

## I. INTERACTION BETWEEN COMPONENTS OF ENERGY

We discuss the interaction between some energy in spin turbulence (ST). Since we do not include any dissipative mechanism, the total energy is conserved. The total energy is the sum of kinetic, trapping potential, spin-independent interaction, and spin-dependent interaction energy; each energy component is not conserved and exchanges with others.

Figure 1 is a typical example showing the time-dependence of each energy component in the case of counterflow corresponding to Fig.1 in the manuscript. In this case, there are the kinetic energy $E_{\rm k}$, spin-independent interaction energy $E_{\rm n}$ and spin-independent interaction energy $E_{\rm s}$, given by

$$E_{\rm k} = \int \sum_{m=-1}^{1} \psi_m^* \left( -\frac{\hbar^2}{2M}\Delta \right) \psi_m d\boldsymbol{r}, \quad (1)$$

$$E_{\rm n} = \frac{c_0}{2} \int n^2 d\boldsymbol{r}, \quad (2)$$

$$E_{\rm s} = \frac{c_1}{2} \int \boldsymbol{s}^2 d\boldsymbol{r}. \quad (3)$$

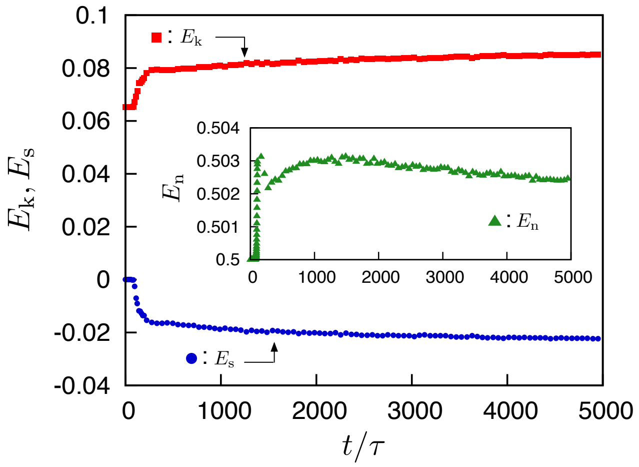


FIG. 1: (Color online) Time-dependence of kinetic, spin-independent interaction and spin-dependent interaction energy in the case of counterflow instability corresponding to Fig.1 in the manuscript. The unit of the energy in the graph is $Nc_0n_0$

The absolute value of $E_{\rm s}$ monotonously increases because of the ferromagnetic interaction ($c_1 < 0$) and the counterflow instability. On the other hand, $E_{\rm n}$ is almost constant owing to the large coefficient $c_0$. As a result, the conservation of the total energy increases $E_{\rm k}$ through the interaction with $E_{\rm s}$. This increase of $E_{\rm k}$ can be related to the fact that the superfluid velocity is induced by the spatial gradient of spin vector and nematic tensor [1], which can affect the configuration of kinetic energy spectrum as discussed in Sec. III.

The detail of the time dependence of energy components depends on each case (the counterflow instability, the instability of spin helical structure in a trapped system and the application of an oscillating magnetic field in a uniform system), but in any case $E_{\rm s}$ interacts with other energy components.

## II. DISSIPATIVE MECHANISM IN ST

This section discusses the dissipative mechanism for $E_{\rm s}$ in ST, which is important for the understanding of ST. When we consider dissipative mechanism in ST, we have to note two things in order to avoid some possible confusion. Firstly, we do not introduce any dissipative mechanism to our system, so that the total energy is conserved. Secondly, the spin-dependent interaction energy $E_{\rm s}$ is not conserved, so we may say that $E_{\rm s}$ can dissipate through the interaction with other components of energy. And this dissipative mechanism may play an important

role to sustain the $-7/3$ power law for the spectrum of $E_{\rm s}$.

In classical turbulence (CT), the kinetic energy in the wave number region higher than the Kolmogorov scale dissipates by the viscosity. If this kind of dissipation is absent, the spectrum in the high wave number region grows and the Kolmogorov $-5/3$ power law is disturbed. Thus, the dissipative mechanism is important for the appearance of the $-5/3$ power law.

In our ST, we numerically confirm the tendency of the accumulation of spin-dependent interaction energy in the high wave number region, which is shown in Fig. 13 (c) and (d) of [2]. Then, the $-7/3$ power law still appears clearly, but can be disturbed if the energy is more accumulated in the high wave number region. This seems to be related to the dissipative mechanism in ST. In conclusion, at present, we do not sufficiently understand the dissipative mechanism in ST. However, we can think of two possibilities.

The first possibility is that the energy is transferred to other energy components. As discussed in Sec. I, the total energy is conserved, but the spin-dependent interaction energy temporally changes through the interaction with other energy components. Thus, In the wave number region higher than $2\pi/\xi_s$, the spin-dependent interaction energy may dissipate through transferring to other components, which leads to the clear $-7/3$ power law. In this high wave number region, the dynamics can reflect the structure and motion of spin vortices and domain walls, which may be important for the dispersive mechanism.

The second possibility is that the energy does not dissipate. If the energy flux is weak, it takes long time to accumulate the energy in the high wave number region. Thus, we may not see the remarkable accumulation because the calculation time is shorter than the time characteristic of the energy flux. This may be related to the slowdown by the dispersive effects [3]. Therefore, the $-7/3$ power law may be disturbed if we run the numerical calculation for a much longer time.

We do not numerically or theoretically confirm these possibilities because the kinetic energy spectrum in the ST is not studied in detail and this mechanism can be related to the interaction between the spin density vector and superfluid velocity.

## III. SPECTRUM OF KINETIC ENERGY

The spectrum of the kinetic energy can be affected by the dynamics of spin density vector because the spatial gradient of the spin density vector induces the superfluid velocity. Actually, in the ferromagnetic state, there is the Mermin-Ho relation which gives the relation between the rotation of the velocity and the gradient of spin vector

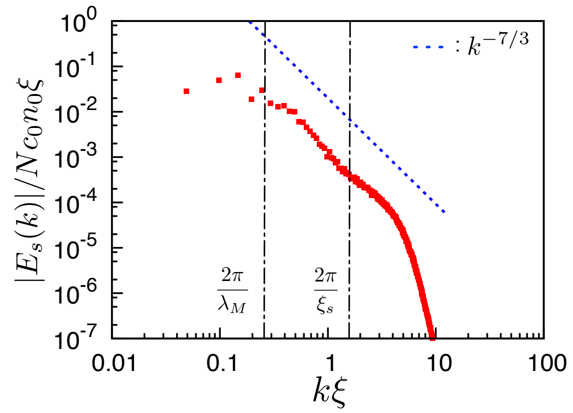


FIG. 2: (Color online) Spectrum of spin-dependent interaction energy obtained by oscillating magnetic field (case of (c)) at $t/\tau = 4000$, when the magnetic field continues to be applied.

[4], which is expressed by

$$\nabla \times \boldsymbol{v} = \frac{\hbar}{2M}\epsilon_{\mu\nu\lambda}\bar{s}_\mu(\nabla\bar{s}_\nu \times \nabla\bar{s}_\lambda), \tag{4}$$

where $\bar{\boldsymbol{s}} = \boldsymbol{s}/n$ is spin density vector normalized by the total density $n$, and $\boldsymbol{v}$ is a superfluid velocity given by

$$\boldsymbol{v} = \frac{\hbar}{2M\rho i}[\psi_m^*\nabla\psi_m - \psi_m\nabla\psi_m^*]. \tag{5}$$

Here, the Greek indices that appear twice are to be summed over $x$, $y$, $z$, and Roman indices are to be summed over $-1$, 0, 1. This is remarkably different from one-component BECs, where the vorticity vanishes without the quantized vortex. Therefore, the gradient of spin density vector induces the superfluid velocity, which may lead to the another power law in the kinetic energy spectrum different from the Kolmogorov $-5/3$ power law because the inertial term $(\boldsymbol{v}\cdot\nabla)\boldsymbol{v}$ is important for the $-5/3$ power law. This is another interesting future work.

We note that Eq. (4) is valid in the ferromagnetic state. The generalized Mermin-Ho relation in the spin-1 spinor GP equation is discussed in [1], where the nematic tensor is introduced and this spatial gradient also induces the superfluid velocity. However, if the spin-dependent interaction is ferromagnetic, the system can be approximately described as the ferromagnetic state. Thus, it is meaningful to discuss the interaction between superfluid velocity and spin density vector in the system with ferromagnetic interaction by using Eq. (4).

## IV. SCALE OF ENERGY INJECTION

In this paper, we obtain ST by using three methods: (a) counterflow instability in a uniform system, (b) instability of the initial helical structure of the spin density

vector in a trapped system and (c) application of an oscillating magnetic field in a uniform ferromagnetic system. This section describes the scale of energy injection in each cases.

In the case (a), we apply the counterflow between the $m = 1$ and $-1$ components at the initial state, so that the energy is injected only at $t = 0$. The counterflow induces the instability with a characteristic length corresponding to the scale of energy injection. This instability is previously studied by using the Bogoliubov de-Gennes equation whose analysis finds this wave number. Actually, the spectrum shows the peak at this wave number as shown in Fig. 13 (a) of [2] when the instability occurs.

In the case (b), we prepare the spin helical structure as the initial state. The wave number of the helical structure corresponds to the scale of energy injection. Actually, the spectrum of spin-dependent interaction energy has a peak at this wave number, which is confirmed in Fig. 3 (a) of [5].

In the case (c), the oscillating magnetic field is applied to obtain the ST. This magnetic field can make the spin structure with a scale characteristic of the field, whose expression is obtained by the resonant condition. In the ferromagnetic state, the dispersion relation of the spin wave is free-particle like. Thus, we obtain the expression $k_M = \sqrt{2M\omega_M/\hbar}$ by the condition $\hbar\omega = \hbar^2 k_M^2/2M$, where $\omega$ is the frequency of the oscillating magnetic field. Actually, the spectrum obtained by this method bends at $k_M$ as shown in Fig. 2.

## V. MAGNITUDE OF MAGNETIZATION $|\boldsymbol{m}(t)|$

We comment on the magnetization $|\boldsymbol{m}(t)|$. In our numerical calculation without the magnetic field, the spatial integral for the spin density vector $\boldsymbol{s}$ is conserved, but that for the normalized spin density vector $\hat{\boldsymbol{s}}$ is not. In the cases for Figs. 3 (a) and (b) in the manuscript, $[\boldsymbol{s}(\boldsymbol{r}, t = 0)]$ at the initial state is almost zero. Thus, because the direction of two vectors is same, the magnetization $|\boldsymbol{m}(t)|$ becomes almost zero. On the other hand, in the case of Fig. 3 (c) in the manuscript,, $[\boldsymbol{s}(\boldsymbol{r}, t = 0)]$ is unity, but the the instability induced by the oscillating magnetic field leads to $[\boldsymbol{s}(\boldsymbol{r}, t)] \sim 0$. Therefore, $|\boldsymbol{m}(t)|$ becomes almost zero too.


[1] E. Yukawa and M. Ueda, Phys. Rev. A **86**, 063614 (2012).
[2] K. Fujimoto and M. Tsubota, Phys. Rev. A **85**, 033642 (2012).
[3] G. Krstulovic and M. Brachet, Phys. Rev. Lett, **106**, 115303 (2011).
[4] Y. Kawaguchi and M. Ueda, Phys. Rep. **520**, 253 (2013).
[5] K. Fujimoto and M. Tsubota, Phys. Rev. A **85**, 053641 (2012).
